# Supplementary material for: Manipulating Andreev and Majorana Bound States with microwaves
Source: arXiv:1411.6885 source file (2015-07-30)
Supplement: Supplementary file 1 [file supplementary.pdf]

# Supplementary Material to
# Manipulating Andreev and Majorana Bound States with microwaves

Joseph Weston,[1,2] Benoit Gaury,[1,2] and Xavier Waintal[1,2]

[1] *Univ. Grenoble Alpes, INAC-SPSMS, F-38000 Grenoble, France*
[2] *CEA, INAC-SPSMS, F-38000 Grenoble, France*

## NUMERICAL SIMULATIONS

*Discretized model.* In order to perform numerical simulations, we first need to obtain a discretized version of our model, Eq. (9) in the main text. First we rescale the energy and momentum by $m^*\alpha^2/2$ and $m^*\alpha$ respectively so that lengths and times are measured in units of $\hbar/m^*\alpha x$ and $2\hbar/m^*\alpha^2$ respectively. Unless otherwise specified, all quantities in this supplementary material are expressed in terms of units derived from these. We discretize the Hamiltonian using a standard central difference approximation for the first and second derivatives with a discretization step $a$: $\partial\Psi/\partial y \approx [\Psi(y+a) - \Psi(y-a)]/(2a)$ and $\partial^2\Psi/\partial y^2 \approx [\Psi(y+a)+\Psi(y-a)-2\Psi(y)]/a^2$ and arrive at the discretized Hamiltonian:

$$\hat{H} = \sum_{i,j=-\infty}^{\infty} c_i^\dagger H_{i,j} c_j \tag{1}$$

with the matrix $H_{i,j}(t)$ containing diagonal and nearest neighbours matrix elements,

$$H_{j,j}(t) = (\frac{2}{a^2} - E_F + U_j)\tau_z + E_z\sigma_z + \Delta_j\tau_x + \delta_{j0}\frac{V_t}{a}\tau_z \tag{2}$$

$$H_{j,j+1}(t) = \left[\frac{1}{a^2}\tau_z + \frac{i}{a}\sigma_x\tau_z\right] T_j(t) \tag{3}$$

$$T_j(t) = \cos[\phi(t)\delta_{j,-l}] + i\tau_z \sin[\phi(t)\delta_{j,-l}] \tag{4}$$

where $c_j^\dagger \equiv \Psi^\dagger(ja) = (\psi_\uparrow^\dagger(ja), \psi_\downarrow^\dagger(ja), \psi_\downarrow(ja), -\psi_\uparrow(ja))$ (and $c_j$, its Hermitian conjugate) are vectors of creation (annihilation) operators at site $j$. $\Delta_j = \Delta$ for $j > L_s/a$ and 0 otherwise and $\phi(t) = \int_0^t dt\, V(t)$. $l = L_N/a$, $U_j$ is 0 for $j < 0$ and $j > L_S/a$, and is otherwise sampled from a uniform random distribution on the interval $[-U/2, U/2]$, where $U$ characterizes the strength of the Anderson disorder. Note that we are working in a gauge where the changing voltage in the normal lead appears as a phase factor multiplying the hopping term at the voltage drop (see Ref. 1 for details). The Pauli matrices $\sigma_i$ and $\tau_i$ respectively act on the spin and electron-hole degrees of freedom.

*Numerical technique.* In order to obtain time-dependent observables, we use the usual out of equilibrium Keldysh formalism. However, in order to make the numerical calculations feasable, we use an alternative formulation as explained in Ref. 1. The Hamiltonian is time-independent for $t < 0$ where the scattering states $\Psi_{\alpha E}^{st}$ (incoming mode $\alpha$ at energy $E$) of the system can be calculated using standard techniques[2]. In our case, we use the Kwant software to obtain them. The scattering states can then be evolved for $t > 0$ by solving the Schrödinger equation,

$$i\partial_t \Psi_{\alpha E}(t) = H(t)\Psi_{\alpha E}(t) \tag{5}$$

with $\Psi_{\alpha E}(0) = \Psi_{\alpha E}^{st}$. The differential conductance is then given by a direct extension of the Landauer formula to the time domain,

$$\frac{dI(t)}{dV} = \frac{2e^2}{h}\Im\sum_\alpha \int dE \frac{\partial f_\alpha(E)}{\partial E} \Psi_{\alpha E}^*(0,t) H_{0,1}(t) \Psi_{\alpha E}(1,t) \tag{6}$$

where $f_\alpha$ is the Fermi distribution with chemical potential $eV$ for the normal lead and $\Im$ denotes the imaginary part. In practice Eq.(5) is still inappropriate for numerical calculations as $H(t)$ is an infinite matrix. Hence, we study the deviation $\bar{\Psi}_{\alpha E}(t)$ from the stationary value, $\Psi_{\alpha E}(t) = \Psi_{\alpha E}^{st} e^{-iEt} + \bar{\Psi}_{\alpha E}(t)$ which follows

$$i\partial_t \bar{\Psi}_{\alpha E}(t) = H(t)\bar{\Psi}_{\alpha E}(t) + [H(t) - H(0)]\Psi_{\alpha E}^{st} e^{-iEt} \tag{7}$$

which can be solved on a finite system since $\bar{\Psi}_{\alpha E}(t = 0) = 0$ and the source term only lies in the small central region.

Details and proofs can, again, be found in Ref. 1.

## DC CHARACTERIZATION

Before performing the time-dependent simulations, DC simulations were carried out using the Kwant quantum transport package[2]. The numerics were used to characterize the (topological or not) regime of the system described by Eq. (1). These results agree perfectly with the findings of Ref. 3.

Fig. 1 shows how the band structure of the (discretized) Hamiltonian changes when successive ingredients are added. Fig. 1c) and Fig. 1d) correspond to the band structures in the normal lead ($y < L_N$) and superconducting lead ($y > L_S$). In the normal lead we clearly see the spin-momentum locking characteristic of a quantum spin-Hall phase, while in the superconductor we see a gapped spectrum where the gap at $k = 0$ is dominated by the Zeeman term. These band structures are of the same type as in Ref. 3.

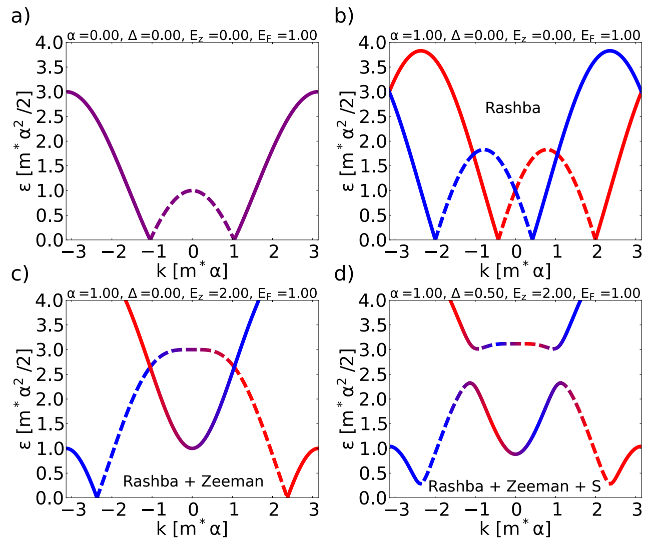


FIG. 1. Band structures of a discrete 1-D infinite chain in the $k > 0$ sector of the Brillouin zone. red/blue coloration (color available online) corresponds to spin up/down and full/dashed lines correspond to electron/hole sectors. a) shows the spectrum for the system without Rashba, Zeeman or superconducting terms; both the spin components are superimposed. b), c) and d) show the addition of these three ingredients in turn.

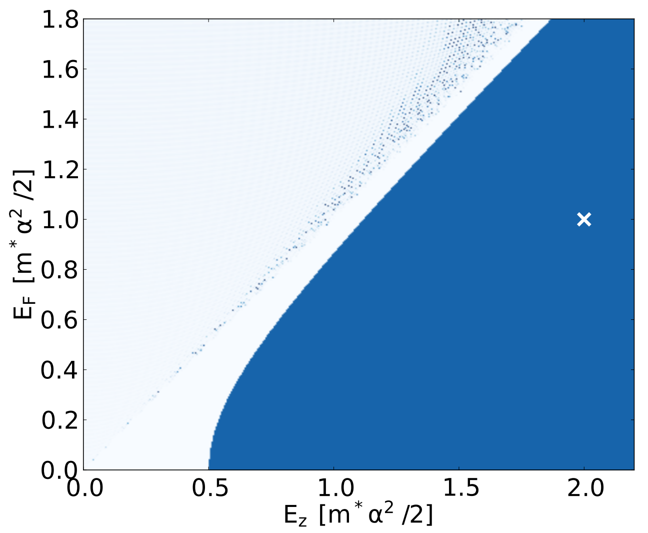


FIG. 2. Colorplot of the zero-bias DC differential conductance (with no time-dependent perturbation) for different values of the Zeeman energy, and Fermi energy. The parameters used were: $\alpha = 1$, $\Delta = 0.5$ and $V_t = 5.0$ ($|d|^2 = 0.17$). The color scale goes between 0 (white) and $2e^2/h$ (blue). The continuous phase where $dI/dV_b = 2e^2/h$ in the $\sqrt{E_z^2 - \Delta^2} \geq E_F$ sector corresponds to a Majorana bound state. The isolated points of high conductance around the $E_z = E_F$ line correspond to regular Andreev bound states crossing zero bias. The white cross indicates where the time-dependent numerical simulations were carried out for the long junction.

Fig. 2 shows a colormap of the zero-bias differential conductance as a function of Zeeman energy (magnetic field) and Fermi energy. The Rashba coupling term is $\alpha = 1$ and the superconducting gap $\Delta = 0.5$. The color-code ranges from 0 (white) to $2e^2/h$ (blue) allowing one to detect the presence of the Majorana mode in the topological phase for $E_F \leq \sqrt{E_z^2 - \Delta^2}$, in agreement with Ref. 3. The conductance in the non-topological region is equal to $|d|^4/(2 - |d|^2)^2$.

## RESULTS IN THE LONG JUNCTION LIMIT

The simple form of Eq. (7) in the main text and the subsequent resonance condition, Eq. (8) in the main text permit an inituitive understanding as outlined in the main text. Figures 3 and 4 show the different contributions to the differential conductance from different orders, $p$. both of these figures were produced from Eq. (7) in the main text using values for the time of flight, $\tau_F$, and barrier transmission amplitude, $d$, obtained from DC simulations of Eq. (1) (without the time-dependent voltage), using Kwant[2]. Fig. 3 clearly shows how the DC resonant peaks are split at finite frequency into components corresponding to the different orders, $p$. Fig. 4e) is a colorplot of the zero bias differential conductance as a function of driving frequency and average number of electrons injected per half-cycle (proportional to driving amplitude). Fig. 4a) - Fig. 4d) show how the different orders $p$ only contribute to resonant peaks at frequencies $q/p$.

## RESULTS IN THE SHORT JUNCTION LIMIT

The long-junction case is useful to understand the mechanism behind the time-dependent effects shown here. In experiment, however, the short-junction case (where the mean level spacing of the resonant junction is of the order of the gap) is more easily accessible. In the experiment of Ref. 4 their junction length of $\sim 200\,\mathrm{nm}$ corresponds (taking the Fermi velocity between $10^4$ to $10^5\,\mathrm{m\,s^{-1}}$) to a mean level spacing, $\delta$, of 50 to $500\,\mu\mathrm{eV}$, i.e. of the order of the superconducting gap, $\Delta$, which was measured to be $250\,\mu\mathrm{eV}$. We performed numerical simulations in this more experimentally relevant regime in order to demonstrate the feasibility of our proposal. We chose $\Delta = 250\,\mu\mathrm{eV}$, $\alpha = 20\,\mathrm{meV\,nm}$ and $E_F = 0$, to match the experimental values of Ref. 4, and a magnetic field of 0.6 T to place us firmly in the topological regime. We used a discretization step of 1 nm, which for the relevant energy scales $\sim \Delta$ gives a band structure that is negligibly different from the continuum limit. Using the above microscopic parameters the Fermi velocity was calculated to be $6.08 \times 10^4\,\mathrm{m\,s^{-1}}$ using kwant, which in principle – for the 100 nm junction used here

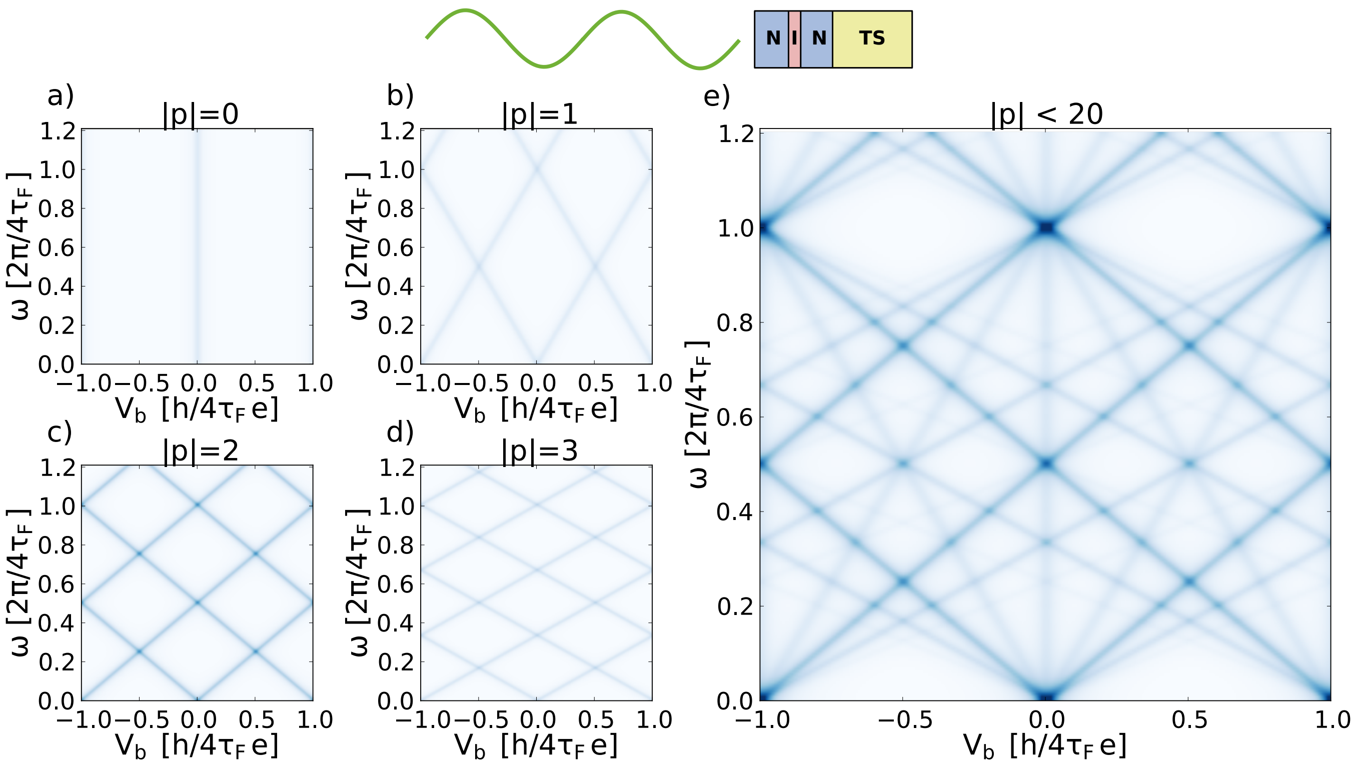


FIG. 3. The contributions to the total differential conductance for different orders $p$ (Eq. (7) in the main text), i.e. $p$-photon processes. a) – d) individual contributions from different orders; contributions from different values of $\omega$ correspond to different values of the integer $q$ (Eq. (8) in the main text). e) The sum of the contributions for all $|p| < 20$, which gives the full differential conductance. A barrier transmission $|d|^2 = 0.17$ was used.

– gives a mean level spacing of 630 µeV. This last condition ensures that we only have the 0-bias resonance present below the gap, as is evident in the experimental data of Ref. 4. In reality resonances close to the superconducting gap are shifted to lower energy due to the energy dependence of the Andreev reflection amplitude, $e^{-i\arccos(E/\Delta)}$.

We performed time-domain simulations for the short-junction system using the parameters presented above. We start with results at zero temperature and without static disorder (purely ballistic sample). Fig. 5a) shows the differential conductance as a function of the bias voltage and driving frequency. The short junction gives a qualitatively different picture than the long junction, however we see that key features of the differential conductance landscape remain. The Majorana peak still splits into several finite-energy peaks at finite frequency, however the contributions from the finite-frequency resonances are largely reduced (in the case of the resonance near the superconducting gap) or even eliminated entirely (for resonances which would be above the superconducting gap).

Fig. 5b) also shows differences from the long-junction case, but maintains some key features. In both Fig. 5a) and Fig. 5b) only the contributions from $q = 0, 1, -1$ are present (corresponding to the DC zero-bias peak and two side-peaks close to the superconducting gap), and fewer $p$ contributions are visible than in the long-junction case. Our analytical treatment from the main text cannot describe this regime, as it was assumed that the transmission/reflection amplitudes ($d$, $r$ and $r_A$) are constant over energy scales $\hbar\omega$ ($\omega$ the driving frequency). As we have $\hbar\omega \sim \Delta$ for the short junction this approximation no longer holds.

An experimental setup used to observe the effect shown here will obviously have to operate at finite temperature, and will be subject to a certain amount of disorder. In Ref. 4 a mean free path of 300 nm was measured, which corresponds to a quasi-ballistic regime. We have conducted microscopic simulations with white-noise disorder to model the experimentally observed regime; the strength of the disorder used gives a mean-free path of 87 nm which, for the 100 nm wires used in our simulations, puts us in the quasi-ballistic regime. The time-dependent simulations shown correspond to a single realisation of disorder but we checked that sample to sample variations do not modify the emerging picture qualitatively. Fig. 6 shows colorplots of the differential conductance at different temperatures with the disorder described above. We see that the shifting of the main resonances is visible up to a temperature of 60 mK, and so should be visible experimentally. It should be emphasised

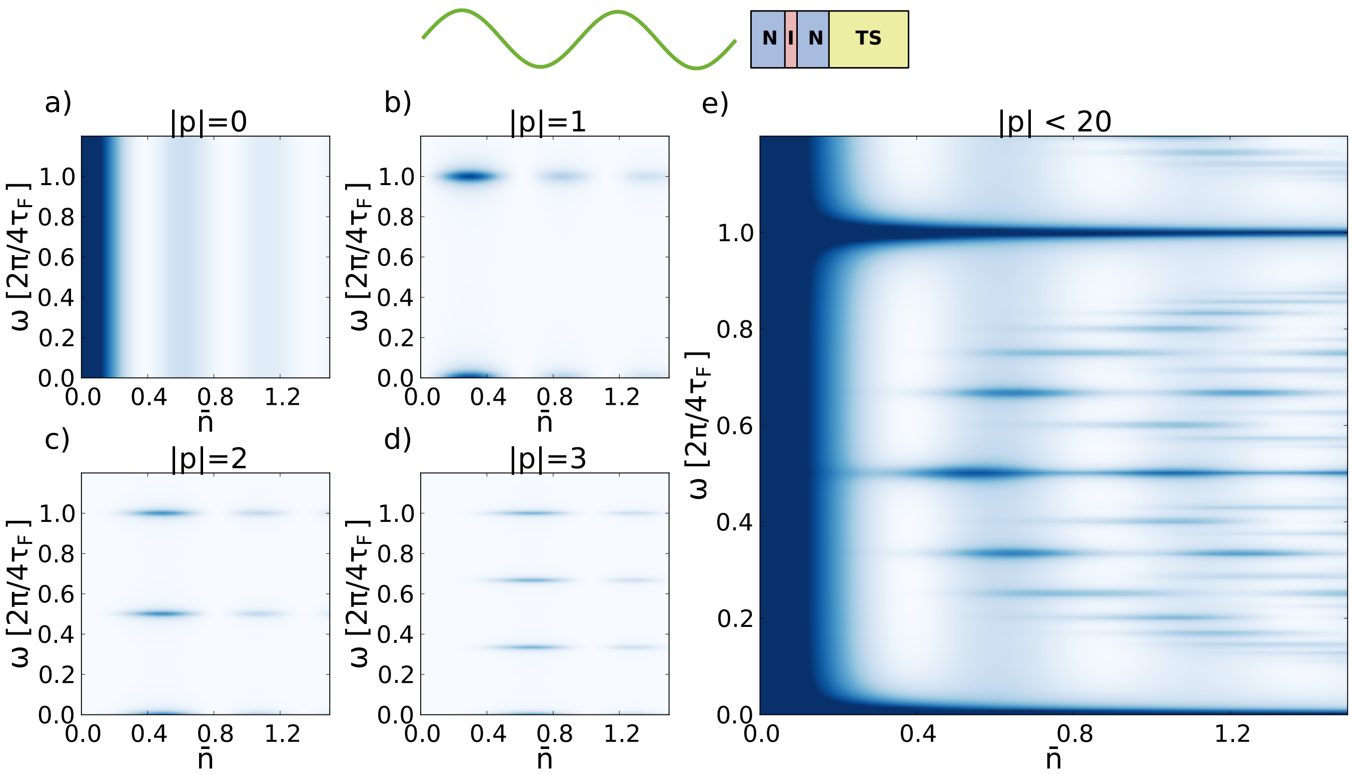


FIG. 4. The contributions to the total differential conductance for different orders $p$ (Eq. (7) in the main text), i.e. $p$-photon processes. a) – d) individual contributions from different orders; contributions from different values of $\omega$ correspond to different values of the integer $q$ (Eq. (8) in the main text). e) The sum of the contributions for all $|p| < 20$, which gives the full differential conductance. A barrier transmission $|d|^2 = 0.17$ was used.

that the addition of the AC bias does not add significant noise to the DC signal; if a resonance is well resolved and visible in a DC experiment then it should also be visible in the presence of AC.

## QUALITATIVE EFFECT OF AC RADIATIONS ON VARIOUS (NON TOPOLOGICAL) SOURCES OF ZERO-BIAS ANOMALY

A direct application of the proposal made in this letter would be to perform the spectroscopy of the zero-bias peaks that form at the edges of a (superconducting) nanowire. Indeed, following the first obervation by Kouwenhoven et al. of zero-bias peaks that could be due to the presence of Majorana bound states, there has been an intense debate both experimental and theoretical on the nature of those peaks. Zero-bias peaks can indeed arise from origins other than topological superconductivity. Below, we quickly review some physical mechanisms leading to zero-bias peaks and discuss qualitatively how they would be affected by AC radiation. We conclude that although their DC signatures might look similar, the presence of radiation would provide clear new elements allowing one to distinguish the Majorana bound states from other effects of different origins.

Let us start by reviewing the observations that one should make upon shining microwaves on a Majorana bound states. On general grounds, adding two new independent parameters to address the physics of the sample (frequency and amplitude of the microwave) can only provide new information on the system, especially as the microwaves affect the system in an highly non linear way.

(A) One should observe a set of resonances for frequencies

$$eV_b + \hbar\omega p = \hbar\omega_0 q \quad (8)$$

where $p$ and $q$ are integers.

(B) The frequency $\omega_0 = \pi/(2\tau_F)$ is proportional to the length of the normal region.

(C) In the absence of Majorana (using, for instance, an in plane magnetic field, to place the system in a non topological regime), one expects a set of resonances at frequencies given by,

$$eV_b + \hbar\omega p = \hbar\omega_0' \left(q + \frac{1}{2}\right) \quad (9)$$

where $\omega_0'$ should be rather close to $\omega_0$ but for the variations of the Fermi group velocity with the pa-

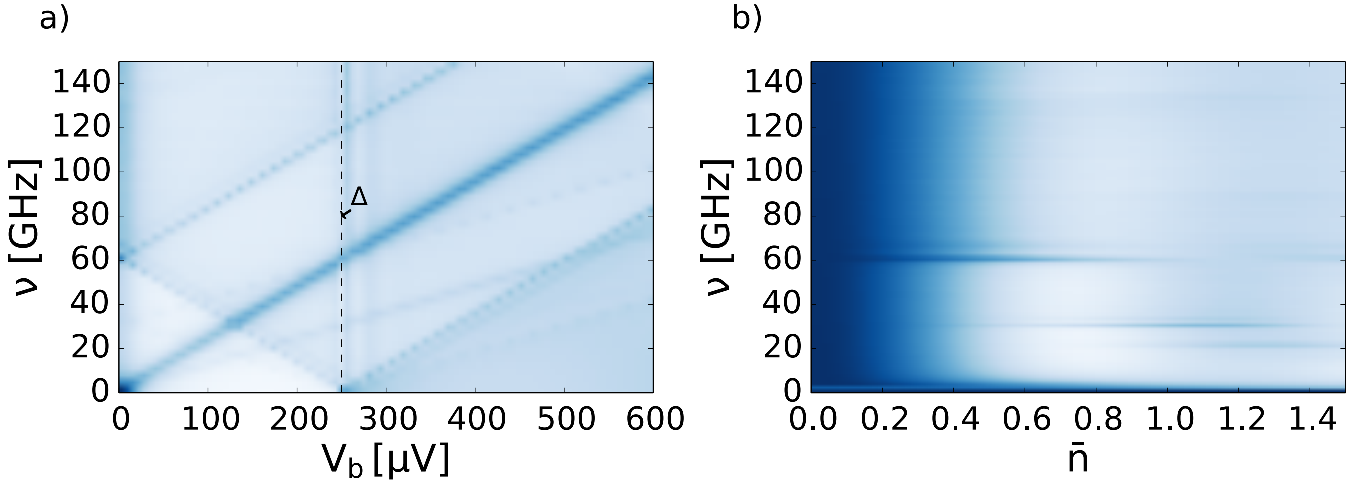


FIG. 5. Differential conductance for the short-junction system in the presence of a sinusoidal voltage at zero temperature and with no disorder. a) Conductance as a function of DC bias, $V_b$, and driving frequency, $\omega$, for $\bar{n} = 0.5$. The dashed line indicates the superconducting gap. b) Conductance as a function of the accumulated phase (divided by $2\pi$) over half a period of the voltage "pulse" train, $\bar{n}$, and the driving frequency $\omega$ at $V_b = 0$. The color scales range from 0 (white) to $2e^2/h$ (blue).

rameter used to tune out the system (e.g. magnetic field). In particular, one recovers a zero-bias anomaly for $\omega = \omega_0'/2$. The factor 1/2 in the previous equation, not present in the topological regime, is a direct manifestation of the $Z_2$ topological invariant.

(D) The amplitude of the resonances has a very peculiar structure with respect to the amplitude of the microwaves, see for instance Fig. 4e)

(E) The characteristic temperature to wash out the resonances is $\hbar\omega_0/k_B$.

(F) The width of the resonances is controled by the tunneling probability to the normal electrode.

Features (A)-(F) put, in our views, very strong constraints on the type of mechanisms that can produce them and should therefore allow one to distinguish between Majorana/Andreev states and other type of resonances. Let us examine a few proposals found in the litterature.

*Kondo resonance.* [5–8] The confining normal region being often rather small, electrostatic repulsion often plays an important role giving rise to Coulomb blockade and possibly Kondo effect. The latter is associated with a zero-bias resonance arising from the electrode electrons that screen the finite spin present in the normal region. The Kondo effect does not have the Fabry-Perot excitation spectrum leading to (A), (C) and (D) so we have no reason to expect these features. Its characteristic energy is the Kondo temperature $T_K$ which depends very sensitively on the electrostatic confinement in contrast to (B). The Kondo temperature also controls the width of the resonance in contrast to (F). In short, while a full description of the effect of AC radiation on the Kondo effect lies outside the scope of the present letter, it is so different from the physics discussed here that the salient features (A) to (F) cannot be found there. In Ref. 6 and 9, the authors observe a differential conductance which shares some features with Majorana physics, yet is attributed to the interplay between superconducting proximity effect and electron repulsion This was also studied theoretically in Ref. 7. Although the physics discussed in Refs. 5, 6, and 9 is continuously connected to the one discussed here (upon increasing the nanowire length), the Coulomb blockade associated with a strong Coulomb repulsion would certainly stop the propagation of the pulses inside the cavity, hence the corresponding dynamical control of the interference pattern a the root of the physics described in this letter.

*Multiple subbands.* It was argued in Ref. 10 that the presence of multiple subbands[11] in conjunction with some disorder and finite temperature can give rise to zero-bias peaks very similar to Majorana peaks[12], even for an even number of bands where the topology of the system is trivial. In contrast to the interacting case discussed above, this situation is a direct extension of the model discussed in this letter and our technique could be used to calculate the spectroscopy in such a case. On a qualitative level, the presence of multiple subbands will have direct consequences on the AC voltage spectroscopy: each subband $\alpha$ has its own Fermi group velocity so that property (A) and (C) are replaced by a set of characteristic frequencies $\omega_0(\alpha)$ and accordingly there would be a much richer spectrum.

*Weak Antilocalization.* Another aspect of multiple sub-bands was studied in Ref. 13. The authors showed

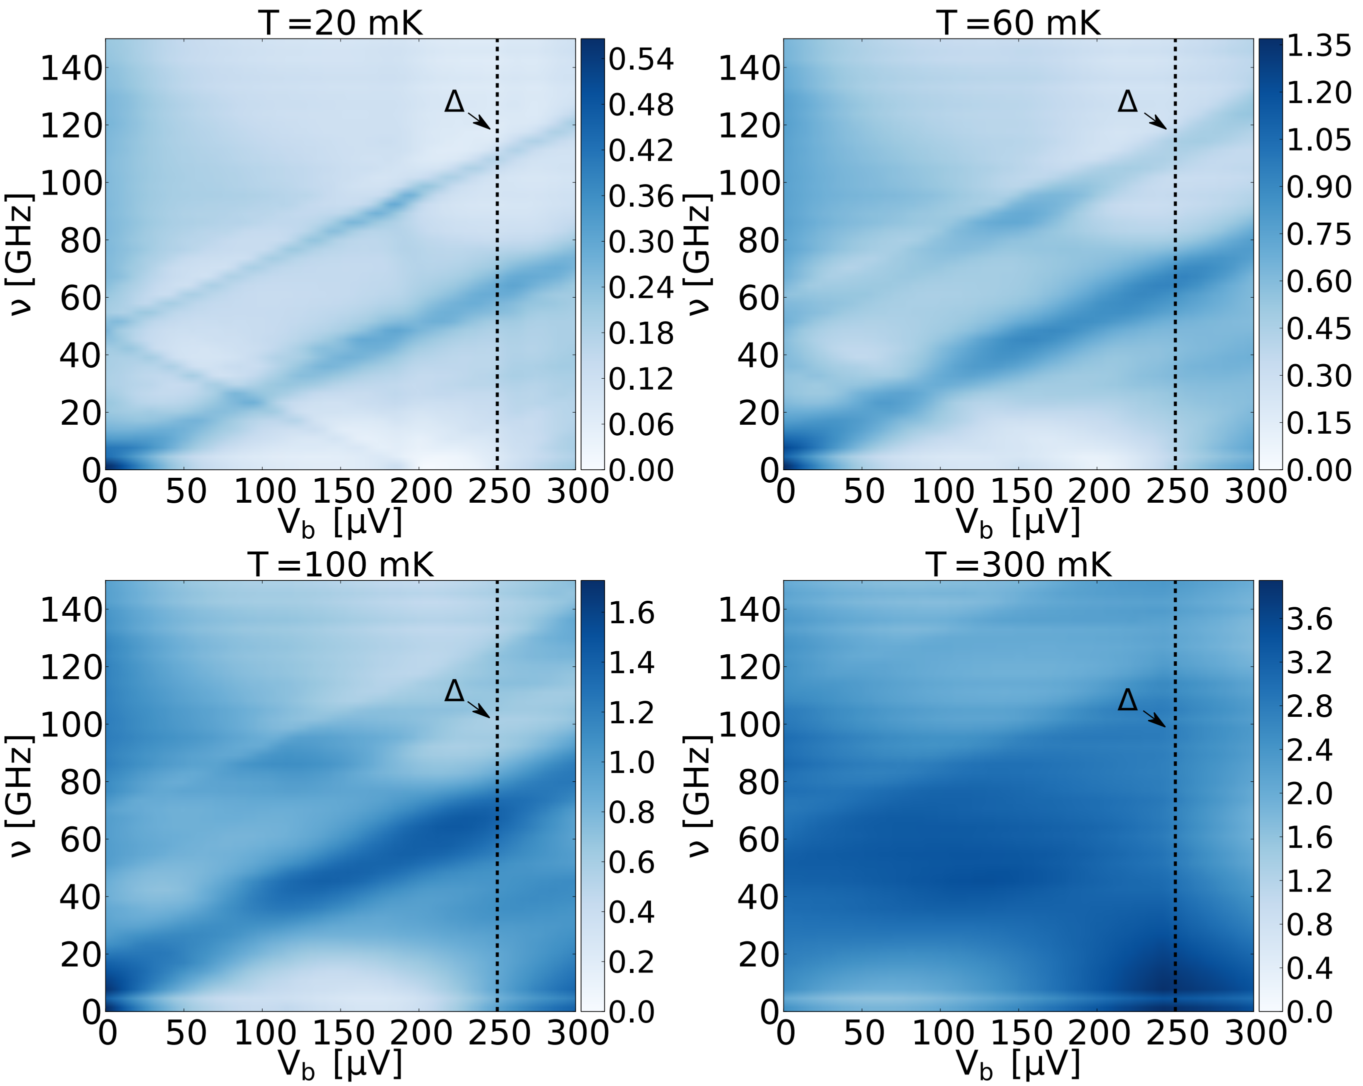


FIG. 6. Differential conductance for the short junction in the presence of disorder and temperature. The colorbars give the color scale for each plot in units of $e^2/h$. The different plots correspond to different temperatures, the vertical dashed lines correspond to the superconducting gap.

that in samples where the Thouless energy was somewhat smaller than the superconducting gap, the effect of weak antilocalization can give rise to a zero-bias peak quite similar to the Majorana one, yet not topologically protected. The physics involved in the presence of weak antilocalization is actually not so different from the one leading to Majoranas so that this mechanism is also not easy to distinguish from genuine Majorana states. A full prediction of the spectroscopy of type of models studied in Ref. 13 would be very interesting and is left for future work. However, we anticipate that a key difference between the Majorana spectrum and the weak anti localization is what happens at the (apparent) quantum critical point: when the zero bias peaks appears (as a function of, say, the magnetic field) one observes a drastic change of the spectrum (property A versus C) in the case of a genuine Majorana. For weak anti localization however, one should observe only a smooth variation of the spectrum with nothing special associated with the appearance of the peak.

*Boundary effects.* A last example involves the role of the boundary of the nanowire. Using a similar model to the one used here, it was shown that when the confining potential of the barrier is smooth, the hybridization of the two non topological zero energy states is exponentially suppressed[14, 15] so that one gets a peak at almost zero bias[16]. A similar effect has also been shown to arise from suppression of the superconducting pair potential and/or enhancement of the Zeeman field at the wire's end[17]. This situation is a bit similar to the weak anti localization mentioned above: the nature of the zero-bias anomaly is not so different from the Majorana one

(in contrast to Kondo effect for instance). We anticipate again that a study of the transition will allow to distinguish between the two cases.

All the examples given above illustrate that the mere presence of a zero bias peaks - even if it is found for the correct regime of direction and strength of the magnetic field expected for Majorana - is not sufficient to establish the presence of a genuine topologically protected state. New probes are needed and we argue that the spectroscopy proposed in this letter, which only involves an additional a.c. voltage while keeping a d.c. measurement, is a simple and efficient one.

[1] B. Gaury, J. Weston, M. Santin, M. Houzet, C. Groth, and X. Waintal, Physics Reports Numerical simulations of time-resolved quantum electronics, **534**, 1 (2014).
[2] C. W. Groth, M. Wimmer, A. R. Akhmerov, and X. Waintal, New J. Phys. **16**, 063065 (2014).
[3] Y. Oreg, G. Refael, and F. von Oppen, Phys. Rev. Lett. **105**, 177002 (2010).
[4] V. Mourik, K. Zuo, S. M. Frolov, S. R. Plissard, E. P. a. M. Bakkers, and L. P. Kouwenhoven, Science **336**, 1003 (2012).
[5] E. J. H. Lee, X. Jiang, R. Aguado, G. Katsaros, C. M. Lieber, and S. De Franceschi, Phys. Rev. Lett. **109**, 186802 (2012).
[6] W. Chang, V. E. Manucharyan, T. S. Jespersen, J. Nygård, and C. M. Marcus, Phys. Rev. Lett. **110**, 217005 (2013).
[7] M. Cheng, M. Becker, B. Bauer, and R. M. Lutchyn, Phys. Rev. X **4**, 031051 (2014).
[8] R. Žitko, J. S. Lim, R. López, and R. Aguado, Phys. Rev. B **91**, 045441 (2015).
[9] E. J. H. Lee, X. Jiang, M. Houzet, R. Aguado, C. M. Lieber, and S. De Franceschi, Nat Nano **9**, 79 (2014).
[10] J. Liu, A. C. Potter, K. T. Law, and P. A. Lee, Phys. Rev. Lett. **109**, 267002 (2012).
[11] R. M. Lutchyn, T. D. Stanescu, and S. Das Sarma, Phys. Rev. Lett. **106**, 127001 (2011).
[12] G. Kells, D. Meidan, and P. W. Brouwer, Phys. Rev. B **85**, 060507 (2012).
[13] D. I. Pikulin, J. P. Dahlhaus, M. Wimmer, H. Schomerus, and C. W. J. Beenakker, New J. Phys. **14**, 125011 (2012).
[14] M.-T. Rieder, G. Kells, M. Duckheim, D. Meidan, and P. W. Brouwer, Phys. Rev. B **86**, 125423 (2012).
[15] T. D. Stanescu and S. Tewari, Phys. Rev. B **89**, 220507 (2014).
[16] G. Kells, D. Meidan, and P. W. Brouwer, Phys. Rev. B **86**, 100503 (2012).
[17] D. Roy, N. Bondyopadhaya, and S. Tewari, Phys. Rev. B **88**, 020502 (2013).
